# Supplementary material for: BAE: BERT-based Adversarial Examples for Text Classification
Source: arXiv:2004.01970 source file (2020-10-08)
Supplement: Supplementary file 2 [file datasets_table.tex]

\begin{table}[t]

\centering
\resizebox{\linewidth}{!}{
\begin{tabular}{ccccc}
\toprule
\textbf{Dataset} & \textbf{\# Classes} & \textbf{Train} & \textbf{Test} & \textbf{Avg Length} \\ \midrule
Amazon           & 2          & 900            & 100           &         10.29            \\ % \hline
Yelp             & 2          & 900            & 100           &         11.66           \\ % \hline
IMDB             & 2          & 900            & 100           &         17.56            \\ % \hline
MR               & 2          & 9595           & 1067          &         20.04          \\ % \hline
MPQA             & 2          & 9543           & 1060          &         3.24          \\ % \hline
Subj             & 2          & 9000           & 1000          &         23.46              \\ % \hline
TREC             & 6          & 5951           & 500           &         7.57            \\  \bottomrule
\end{tabular}
}
\caption{Summary statistics for the datasets}
\label{tab:dataset}
\end{table}
