# Supplementary material for: BAE: BERT-based Adversarial Examples for Text Classification
Source: arXiv:2004.01970 source file (2020-10-08)
Supplement: Supplementary file 3 [file supp_graphs.tex]

% \setlength{\floatsep}{-10pt}

%%% AMAZON
\begin{figure*}[h!]
    \begin{subfigure}[h]{0.2\textwidth}
        \includegraphics[width=\textwidth]{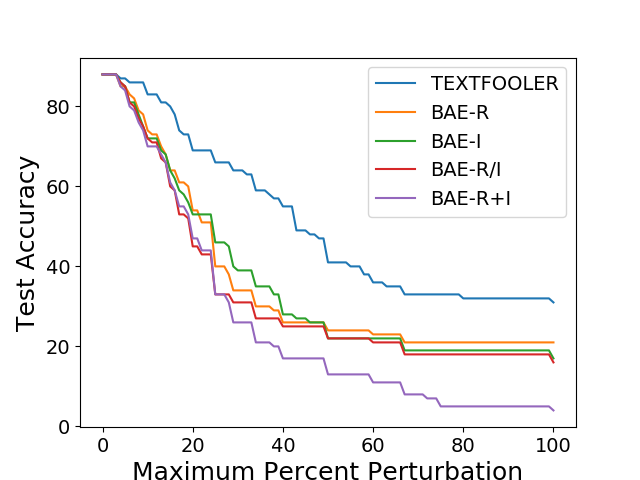}
        \caption{Word-LSTM}
    \end{subfigure}
    \begin{subfigure}[h]{0.2\textwidth}
        \includegraphics[width=\textwidth]{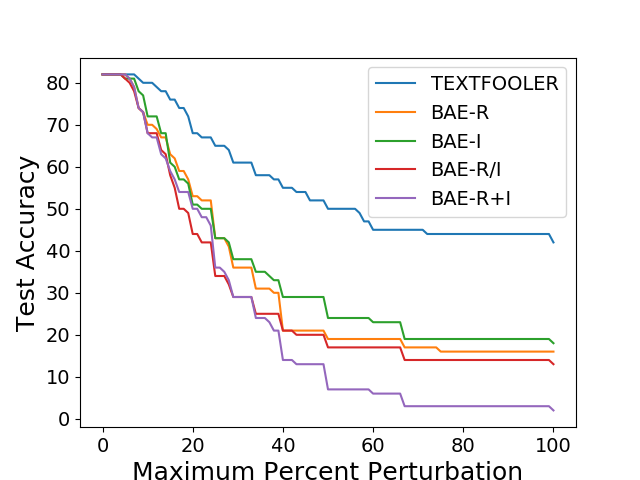}
        \caption{Word-CNN}
    \end{subfigure}
    \begin{subfigure}[h]{0.2\textwidth}
        \includegraphics[width=\textwidth]{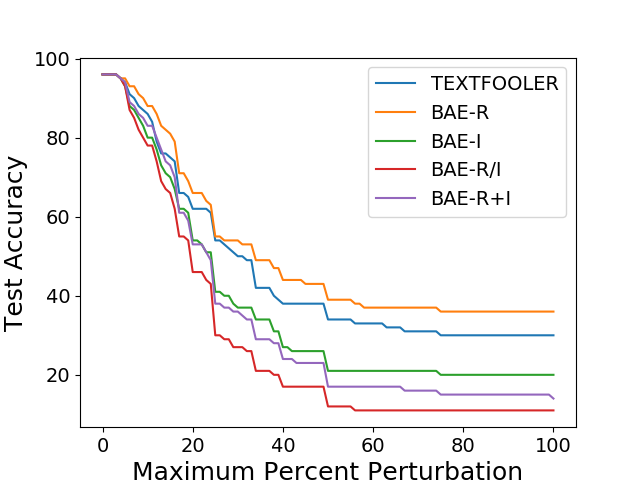}
        \caption{BERT}
    \end{subfigure}
    \vspace{-8pt}
    \caption{Amazon}
    \label{app:graph_amazon}
\end{figure*}   

\vfill

% \vspace{}

%%% Yelp
\begin{figure*}[h]
    \begin{subfigure}[h]{0.2\textwidth}
        \includegraphics[width=\textwidth]{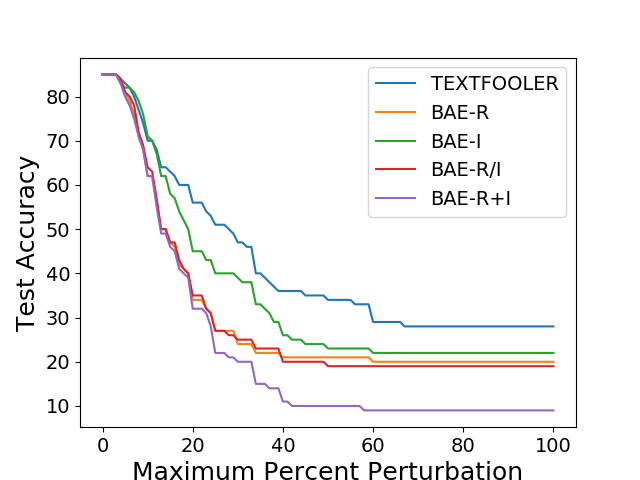}
        \caption{Word-LSTM}
    \end{subfigure}
    \begin{subfigure}[h]{0.2\textwidth}
        \includegraphics[width=\textwidth]{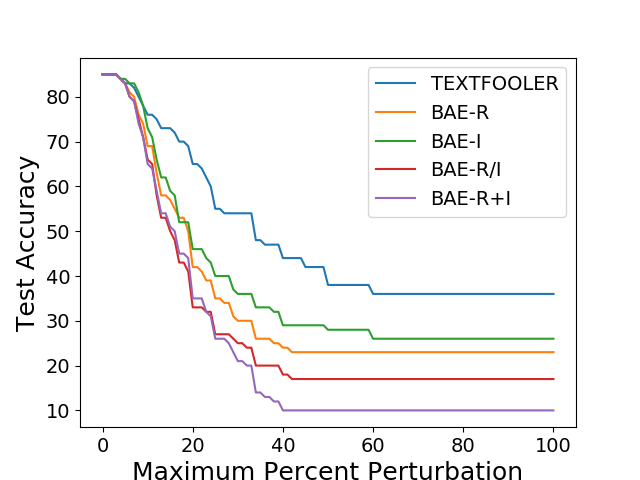}
        \caption{Word-CNN}
    \end{subfigure}
    \begin{subfigure}[h]{0.2\textwidth}
        \includegraphics[width=\textwidth]{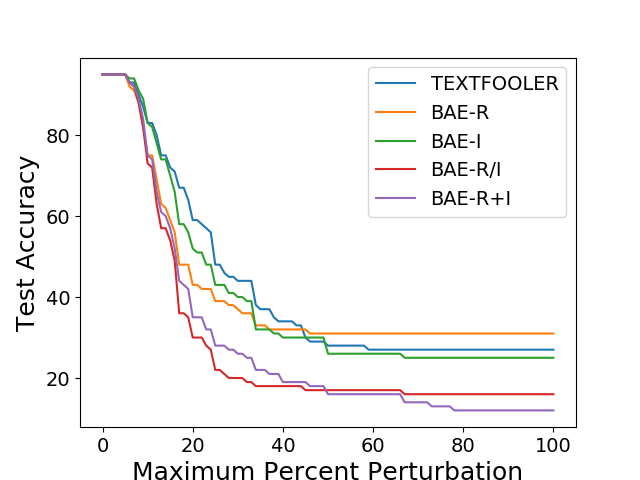}
        \caption{BERT}
    \end{subfigure}
    \vspace{-8pt}
    \caption{Yelp}
\end{figure*}   

\vfill

%%% IMDB
\begin{figure*}[h]
    \begin{subfigure}[h]{0.2\textwidth}
        \includegraphics[width=\textwidth]{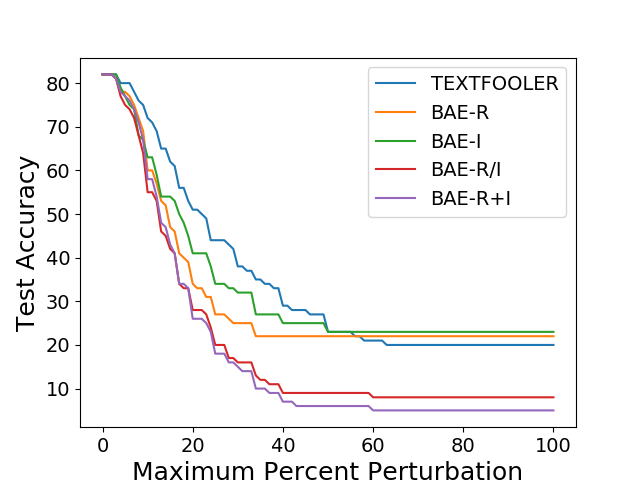}
        \caption{Word-LSTM}
    \end{subfigure}
    \begin{subfigure}[h]{0.2\textwidth}
        \includegraphics[width=\textwidth]{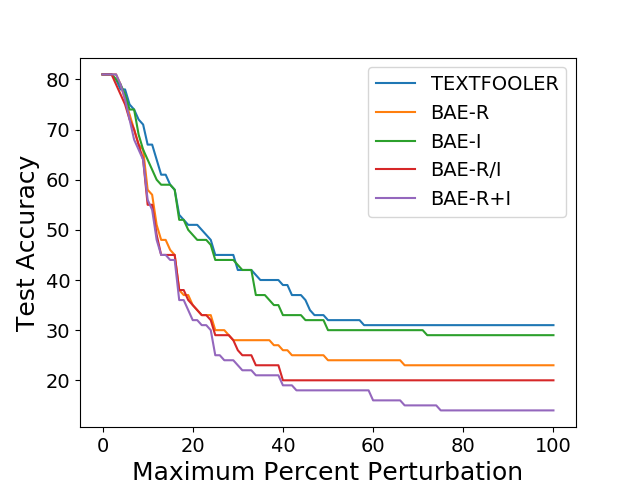}
        \caption{Word-CNN}
    \end{subfigure}
    \begin{subfigure}[h]{0.2\textwidth}
        \includegraphics[width=\textwidth]{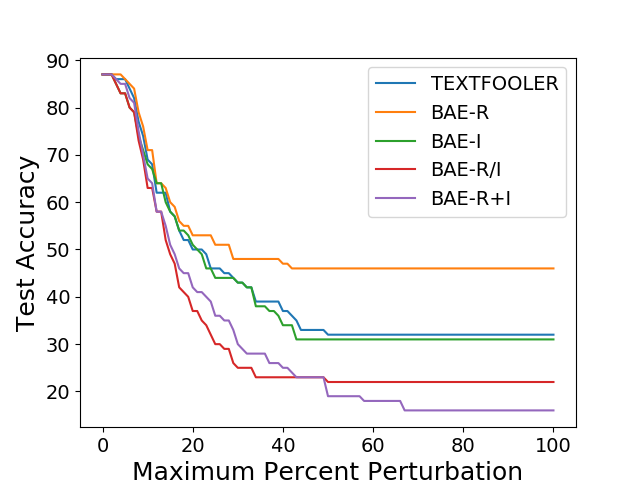}
        \caption{BERT}
    \end{subfigure}
    \vspace{-8pt}
    \caption{IMDB}
\end{figure*}   

\vfill

%%% MR
\begin{figure*}[h]
    \begin{subfigure}[h]{0.2\textwidth}
        \includegraphics[width=\textwidth]{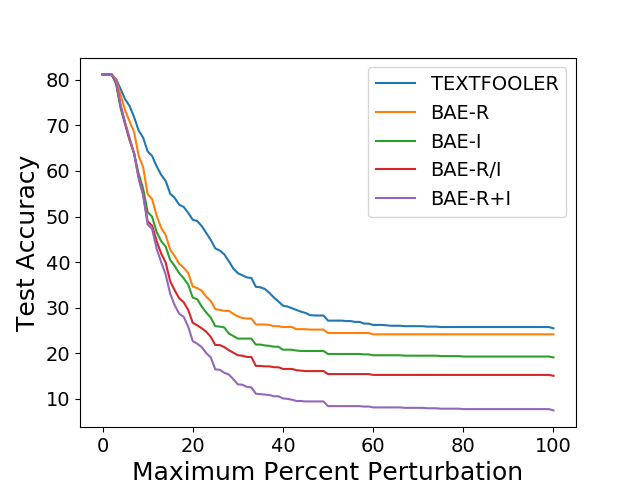}
        \caption{Word-LSTM}
    \end{subfigure}
    \begin{subfigure}[h]{0.2\textwidth}
        \includegraphics[width=\textwidth]{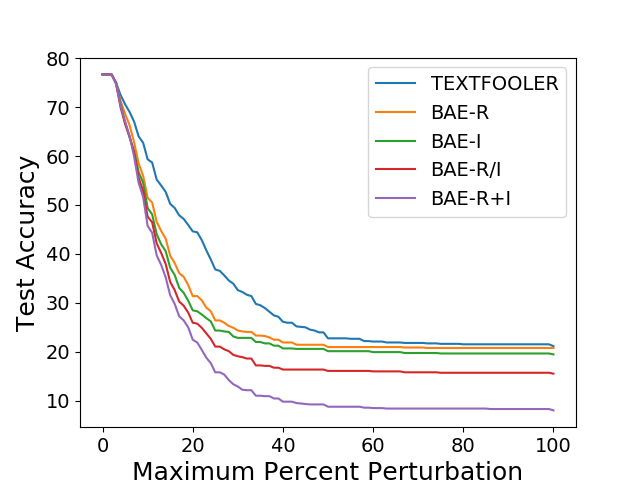}
        \caption{Word-CNN}
    \end{subfigure}
    \begin{subfigure}[h]{0.2\textwidth}
        \includegraphics[width=\textwidth]{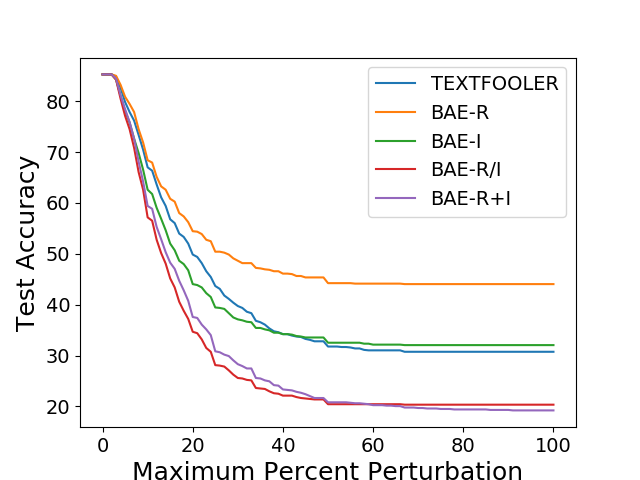}
        \caption{BERT}
    \end{subfigure}
    \vspace{-8pt}
    \caption{MR}
\end{figure*}   

\vfill

%%% MPQA
\begin{figure*}[h]
    \begin{subfigure}[h]{0.2\textwidth}
        \includegraphics[width=\textwidth]{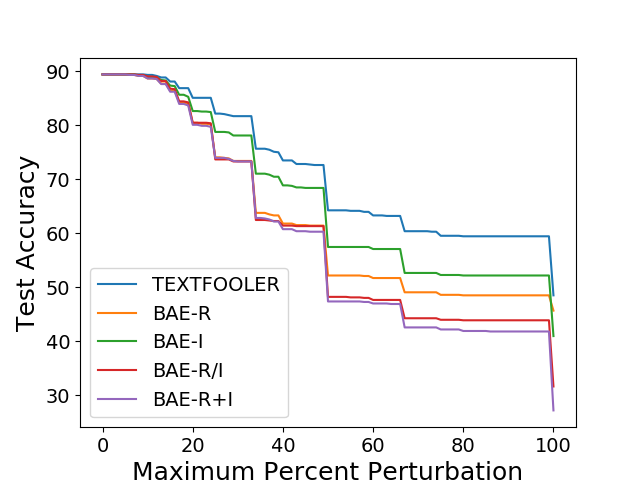}
        \caption{Word-LSTM}
    \end{subfigure}
    \begin{subfigure}[h]{0.2\textwidth}
        \includegraphics[width=\textwidth]{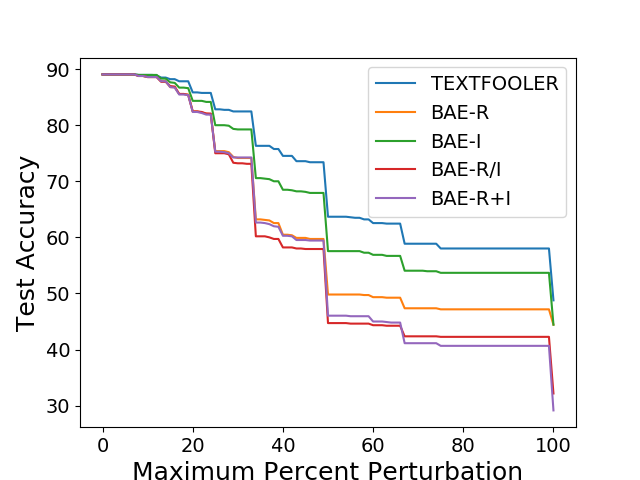}
        \caption{Word-CNN}
    \end{subfigure}
    \begin{subfigure}[h]{0.2\textwidth}
        \includegraphics[width=\textwidth]{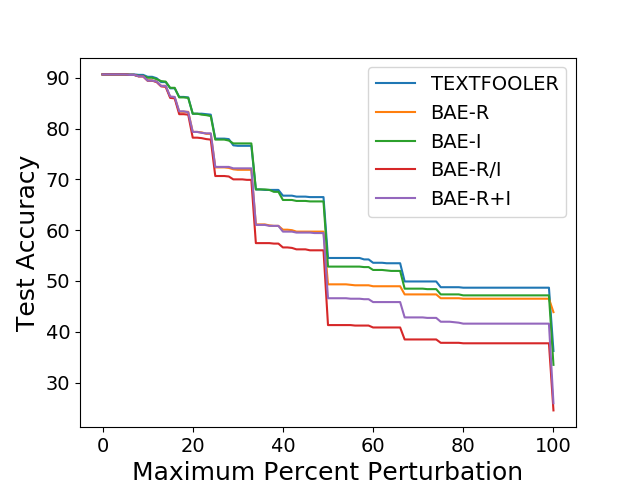}
        \caption{BERT}
    \end{subfigure}
    \vspace{-8pt}
    \caption{MPQA}
\end{figure*}   

\vfill

%%% Subj
\begin{figure*}[h]
    \begin{subfigure}[h]{0.2\textwidth}
        \includegraphics[width=\textwidth]{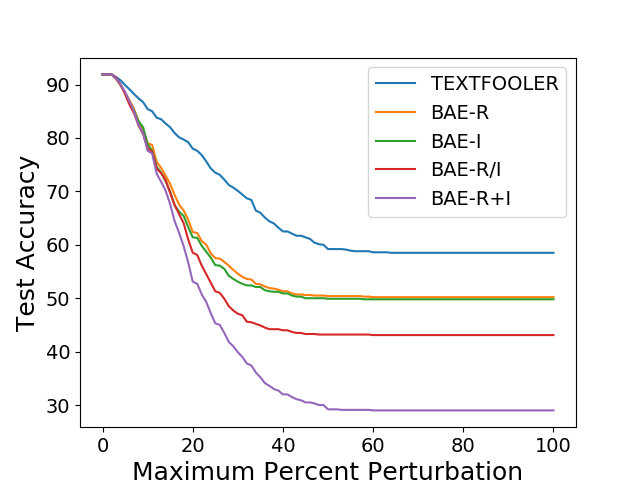}
        \caption{Word-LSTM}
    \end{subfigure}
    \begin{subfigure}[h]{0.2\textwidth}
        \includegraphics[width=\textwidth]{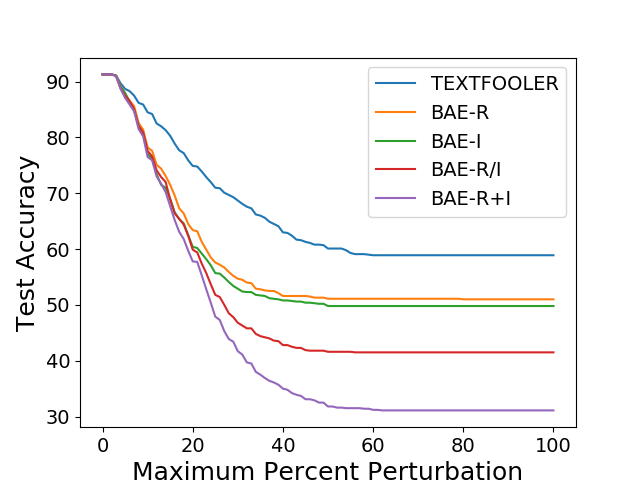}
        \caption{Word-CNN}
    \end{subfigure}
    \begin{subfigure}[h]{0.2\textwidth}
        \includegraphics[width=\textwidth]{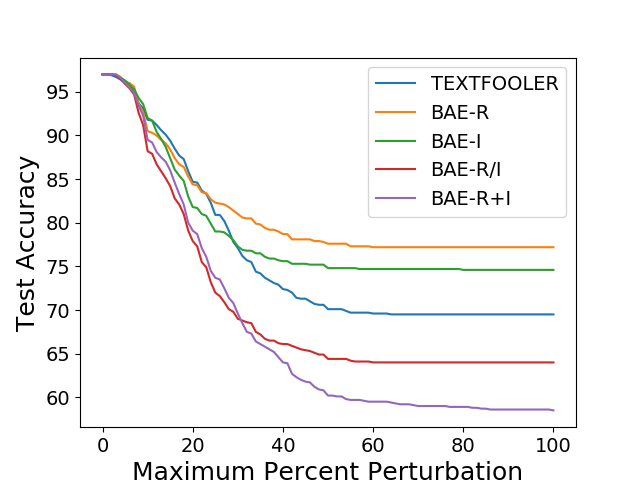}
        \caption{BERT}
    \end{subfigure}
    \vspace{-8pt}
    \caption{Subj}
    \label{app:graph_subj}
\end{figure*}
